# Supplementary material for: Disentangling Generative Factors of Physical Fields Using Variational Autoencoders
Source: arXiv:2109.07399 source file (2021-11-15)
Supplement: Supplementary file 1 [file Appendix_backup.tex]

\appendix
\section{ Governing Equations for Full Order Model}
\label{appendix:fom_eq}

The full order model computations are carried out with an in-house CFD code, the General Equations and Mesh Solver (GEMS), the capabilities of which has been successfully demonstrated in modeling rocket combustion instabilities~\cite{HarvazinskiPoF}. GEMS solves the conservation equations for mass, momentum, energy and species mass fractions in a coupled fashion,
\begin{equation}
    \frac{\partial{Q}}{\partial{t}}+\nabla \cdot\left(\vec{F}-\vec{F_v}\right)=H,
    \label{fom:governing}
\end{equation}
where $Q$ is the vector of conserved variables defined as, $Q=\left(\begin{array}{cccccc}
        \rho & \rho{u} & \rho{v} & \rho{w} & \rho{h^0-p} & \rho{Y_l}\\
    \end{array}\right)^T$
with $\rho$ representing density, $u$, $v$ and $w$ representing velocity field, $Y_l$ representing the $l^{th}$ species mass fraction and the total enthalpy $h^0$ is defined as, $h^0=h+\frac{1}{2}(u^2_i)=\sum_l{h_l{Y_l}}+\frac{1}{2}(u^2_i)$.

The fluxes have been separated into inviscid, $\vec{F}=F_{i}\vec{i}+F_{j}\vec{j}+F_{k}\vec{k}$ and viscous terms, $\vec{F_v}=F_{v,i}\vec{i}+F_{v,j}\vec{j}+F_{v,k}\vec{k}$. And the three inviscid fluxes are,
\begin{equation}
    F_i = \left(\begin{array}{c}
        \rho{u} \\
        \rho{u^2}+p \\
        \rho{uv} \\
        \rho{uw} \\
        \rho{uh^0} \\
        \rho{uY_l} \\
    \end{array} \right), \; F_j = \left(\begin{array}{c}
        \rho{v} \\
        \rho{uv} \\
        \rho{v^2}+p \\
        \rho{vw} \\
        \rho{vh^0} \\
        \rho{vY_l} \\
    \end{array} \right) \; \text{and} \; F_k = \left(\begin{array}{c}
        \rho{w} \\
        \rho{uw} \\
        \rho{vw}+p \\
        \rho{w^2}+p \\
        \rho{wh^0} \\
        \rho{wY_l} \\
    \end{array} \right)
    \label{fom:inviscid_fluxes}
\end{equation}
The viscous fluxes are,
\begin{equation}
    \scalebox{0.8}{$F_{v,i} = \left(\begin{array}{c}
        0 \\
        \tau_{ii} \\
        \tau_{ji} \\
        \tau_{ki} \\
        u\tau_{ii}+v\tau_{ji}+w\tau_{ki}-q_i \\
        \rho{D_{l}}\frac{\partial{Y_l}}{\partial{x}} \\
    \end{array} \right), \; F_{v,j} = \left(\begin{array}{c}
        0 \\
        \tau_{ij} \\
        \tau_{jj} \\
        \tau_{kj} \\
        u\tau_{ij}+v\tau_{jj}+w\tau_{kj}-q_j \\
        \rho{D_{l}}\frac{\partial{Y_l}}{\partial{y}} \\
    \end{array} \right) \; \text{and} \; F_{v,k} = \left(\begin{array}{c}
        0 \\
        \tau_{ik} \\
        \tau_{jk} \\
        \tau_{kk} \\
        u\tau_{ik}+v\tau_{jk}+w\tau_{kk}-q_k \\
        \rho{D_{l}}\frac{\partial{Y_l}}{\partial{z}} \\
    \end{array} \right)$}
    \label{fom:viscous_fluxes}
\end{equation}
where $D_l$ is defined to be the diffusion of the $l^{th}$  species into the mixture. In practice, this is an approximation used to model the multicomponent diffusion as the binary diffusion of each species into a mixture.

The heat flux in the $i^{th}$ direction, $q_i$, is defined as,
\begin{equation}
    q_i = -K\frac{\partial{T}}{\partial{x_i}}+\rho\sum^N_{l=1}D_l\frac{\partial{Y_l}}{\partial{x_i}}h_l+\mathbf{Q}_{\text{source}}
    \label{fom:heat_flux}
\end{equation}
The three terms in the heat flux represent the heat transfer due to the conduction, species diffusion and heat generation from a volumetric source (e.g. heat radiation or external heat source) respectively.

The shear stress, $\tau$ , is also found in the viscous flux and defined in terms of the molecular viscosity and velocity field,
\begin{equation}
    \tau_{ij} = \mu\left(\frac{\partial{u_i}}{\partial{x_j}}+\frac{\partial{u_j}}{\partial{x_i}}-\frac{2}{3}\frac{\partial{u_m}}{\partial{x_m}}\delta_{ij}\right)
    \label{fom:shear_stress}
\end{equation}

The source term, $H$ includes a single entry for each of the species equations signifying the production or destruction of the $l^{th}$ species, $\dot{\omega}_l$, which is determined by the chemical kinetics~\cite{WestbrookDryer},
\begin{equation}
    H=\left(\begin{array}{cccccc}
        0 & 0 & 0 & 0 & 0 & \dot{\omega}_l\\
    \end{array}\right)^T
    \label{cfd:source_term}
\end{equation}

\section{Effects of Unphysical Oscillations in Species Mass Fractions on ROM Development}
\label{appendix:species_oscillations}
